# Supplementary material for: Imaginary time, shredded propagator method for large-scale GW calculations
Source: arXiv:1707.06752 source file (2018-03-07)
Supplement: Supplementary file 1 [file supplement.pdf]

# Supplementary material for "Imaginary time, shredded propagator method for large-scale GW calculations"

Minjung Kim
*Department of Applied Physics, Yale University, New Haven, Connecticut 06520, USA*

Glenn J. Martyna
*IBM TJ Watson Laboratory, Yorktown Heights, New York, USA*

Sohrab Ismail-Beigi*
*Department of Applied Physics, Yale University, New Haven, Connecticut 06520, USA*
(Dated: February 17, 2018)

## INTERPOLATION APPROACH

In real space, the static random phase approximation (RPA) irreducible polarizability matrix is

$$P_{r,r'} = -2\sum_{v}^{N_v}\sum_{c}^{N_c}\frac{\psi^*_{r,v}\psi_{r,c}\psi^*_{r',c}\psi_{r',v}}{E_c - E_v} \tag{1}$$

One advantage of working in a real-space basis is that the sum over products of wave functions is separable so one can come up with cubic scaling algorithms if one can make separable approximations to the energy denominator. We begin by rewriting $P$ as

$$P_{r,r'} = -2\sum_{v}\psi^*_{r,v}\,A(E_v)_{r,r'}\,\psi_{r',v}$$

where the matrix $A$ is defined as

$$A(z)_{r,r'} = \sum_{c}\psi_{r,c}\psi^*_{r',c}/(E_c - z)\,.$$

For a system with an energy gap $E_g$, the denominator $E_c - E_v$ is always positive with a minimum value of the gap $E_g$. Furthermore, the matrix $A$ must be evaluated only for energies $z$ within the range of valence band energies $E_v$. Hence, the calculation of $P$ uses $A(z)$ for values of $z$ where it is smooth in $z$. This means we can use interpolation: we first tabulate $A(z)$ for a range of $z$ values ranging over the valence band energies. This tabulation costs $N_zN_cN_r^2$ which is cubic since the valence band width is an intensive quantity and the number of points $N_z$ needed for a fixed accuracy is a fixed, intensive number. Next, to compute $P$, we sum over $v$, and for each $E_v$ we interpolate $A$ to that energy by using the tabulated $A$. This calculation is also cubic and costs $N_iN_vN_r^2$ where $N_i \le N_z$ is the number of tabulated $z$ values needed for interpolation (e.g., $N_i = 2$ for linear interpolation).

An efficient interpolation scheme should require a small number of $z$ points $N_z$ as well as a modest interpolation cost $N_i$. In our case, the energy dependence requiring interpolation is given by $1/(E_c - z)$ which is most rapidly changing for the largest values of $z$ near the top of the valence $E_v^{max}$ band and when $E_c$ takes on its smallest value at the conduction band minimum $E_c^{min}$. Hence, an efficient interpolation scheme will use a non-uniform $z$ grid that appropriately concentrates sampling points near $E_v^{max}$.

The next section below describes the approach we use to find optimal interpolation grids $z_j$ for the case of linear interpolation (i.e., two-point nearest neighbor interpolation with $N_i = 2$) when sampling over the entire range of valence band energies. We note higher order interpolation schemes with $N_i > 2$ can be used as well that will reduce the number of grid points needed for a fixed error but require more work to perform the interpolation. In our experience, the higher order interpolations do not in the end improve performance at the same level of error when compared to the simpler linear interpolation method.

Regardless of the precise interpolation scheme used, all such interpolation methods will have errors that decrease as a power of the number of grid points $n$. As the data presented in the main text shows, the Laplace transform based methods turn out to have superior error properties (their errors fall off exponentially in $n$).

## ENERGY GRIDS FOR INTERPOLATION

The function of $z$ that we wish to interpolate over $z$ is

$$A(z)_{r,r'} = \sum_{c}^{N_c}\frac{\psi_{r,c}\psi^*_{r',c}}{E_c - z}\,.$$

The function is steepest in $z$ close to the top of the valence band $E_v^{max}$ when the energy difference in the denominator is small. In fact, we will consider the worse case scenario and focus on the stiffest and steepest term in the entire sum which is for the case $E_c = E_c^{min}$, the conduction band minimum energy. Hence the most dif-

ficult to interpolate term is given by the dimensionless function

$$f(z) = \frac{E_{gap}}{E_c^{min} - z} \equiv \frac{1}{1+x},$$

where $z = E_v^{max} - xE_{gap}$, and the scaled energy variable $x$ satisfies $0 \leq x \leq (E_v^{max} - E_v^{min})/E_{gap}$.

The question is how to pick a grid of $\{x_j\}$ values with $n$ points where $x_1 = 0$ and $x_n = (E_v^{max} - E_v^{min})/E_{gap}$. For simplicity, we will be using linear interpolation, so that given some $x$ between two grid points $x_j \leq x \leq x_{j+1}$, the linear interpolation is $f^l(x) = [f(x_j)(x_{j+1} - x) + f(x_{j+1})(x - x_j)]/\Delta x_j$ where $\Delta x_j = x_{j+1} - x_j$. Calculus then provides an analytical expression for the maximum error $f^l(x) - f(x)$ in the interval $x_j \leq x \leq x_{j+1}$. For large $n$ and thus small spacings $\Delta x_j$, the lowest order term for the error is

$$(f^I - f)_{max} \approx \frac{(\Delta x_j)^2}{4(1+x_j)^3}\,.$$

We wish to bound this error by a fixed tolerance $\epsilon$ for all $j$,

$$\frac{(\Delta x_j)^2}{4(1+x_j)^3} \leq \epsilon\,. \tag{2}$$

which then in principle determines the grid points $x_j$. In practice, exact solution of this equation is very difficult, so we again appeal to the large $n$ limit where $x_j$ can be viewed as a function $x(j)$ of a continuous argument $j$ so we approximate $\Delta x_j \approx dx/dj$. Then Eq. (2) turns into an ordinary differential equation with specified boundary conditions. The solution is

$$x(j) = \frac{1}{(1-(j-1)\sqrt{\epsilon})^2} - 1\,.$$

Since $x(n) = (E_v^{max} - E_v^{min})/E_{gap}$ is known, this determines $n$ for each $\epsilon$. And finally we have $z_j = E_v^{max} - x_j E_{gap}$.

The above choice of grid bounds the error when evaluating the function once. However, when using the interpolation to compute $P$ from $A$, we will be evaluating the interpolation over many values across the valence band which approximate an integral. Hence, a more appropriate error control scheme will not only consider the error in interpolating $f(x)$ but also the fact that narrower intervals of $x$ will be sampled less often (assuming a smooth and roughly flat density of states). Hence we should instead bound the error in the function times the size of the interval:

$$\Delta x_j \times \frac{(\Delta x_j)^2}{4(1+x_j)^3} \leq \epsilon$$

Repeating the above exercise, the grid appropriate to this error bound is given by

$$x(j) = \exp\Big([4\epsilon]^{1/3}(j-1)\Big) - 1\,. \tag{3}$$

As before, the fixed value of $x(n)$ then determines $n$ at fixed $\epsilon$, and we use the $x_j$ to get the energy grid points $z_j$. The results in the main text are based on use of this second (exponential) grid of Eq. (3).

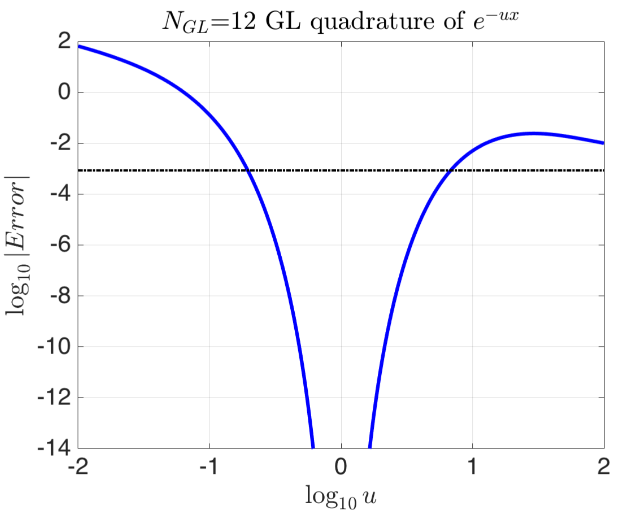


FIG. 1. Error of GL quadrature of $e^{-ux}$ with 12 quadrature points as a function of $u$. The solid blue curve is the error versus $u$. The dashed black horizontal line represents the choice of $a$ giving equal errors at $u = E_{gap}/a < 1$ and $u = E_{bw}/a > 1$ for the case $E_{bw}/E_{gap} = 23$.

## CHOICE OF ENERGY SCALE $a$

We describe how $a \approx \sqrt{E_{bw}/E_{gap}}$ is a very good choice for the energy scale $a$ that minimizes the error of the Gauss-Laguerre (GL) quadrature. Specifically, we are dealing with the GL quadrature of

$$\frac{1}{\Delta} = \frac{1}{a}\int_0^\infty e^{-x\Delta/a}dx \approx \frac{1}{a}\sum_{k=1}^{N_{GL}} w_k e^{-x_k(\Delta/a-1)}$$

where $\Delta = E_c - E_v > 0$ are the interband transition energies. We define the dimensionless $u = \Delta/a$, and the error we wish to minimize is the universal error function

$$Error(u) = \frac{1}{u} - \sum_{k=1}^{N_{GL}} w_k e^{-x_k(u-1)}\,.$$

We note that the error is exactly zero at $u = 1$ since the quadrature is exact when integrating $e^{-x}$. Figure 1 shows a representative plot of the error versus $u$ on a log-log scale. The main point is that the error curve is quite symmetric around $\ln u = 0$ on a logarithmic scale,

especially when smaller error values are of interest (which is the case when we converge results). Namely, the error function, to a good approximation, is even in $\ln u$ about $\ln u = 0$.

The interband energies $\Delta$ range from $E_{gap}$ to $E_{bw}$. Glancing at the Figure 1, the best way to ensure that the lowest errors are sampled as $u$ ranges from its lowest value of $E_{gap}/a$ to its highest value of $E_{bw}/a$ is to choose $a$ such that $u = E_{gap}/a < 1$ and $u = E_{gap}/a > 1$ straddle $u = 1$ and have the same error. For a symmetric error function about $\ln u = 0$, this means we want $-\ln(E_{gap}/a) = \ln(E_{bw}/a)$ which yields $a = \sqrt{E_{bw}/E_{gap}}$. This approximate choice of $a$ becomes exact as $N_{GL}$ is increased and the errors are reduced as well as when $E_{bw}/E_{gap}$ is small.

## ERROR IN GAUSS-LAGUERRE QUADRATURE

We analyze the error made in computing $\hat{P}$ (see main text for its use)

$$\hat{P} = \sum_c \sum_v \frac{1}{E_c - E_v} \tag{4}$$

via Gauss-Laguerre quadrature with $N_{GL}$ points as a function of the band width $E_{bw}$ and band gap $E_{gap}$ of the system. If we require at most a 0.1% error in $\hat{P}$, the resulting $N_{GL}$ is shown versus $E_{bw}/E_{gap}$ in Figure 2. We see that $N_{GL} \propto \sqrt{E_{bw}/E_{gap}}$ is an excellent approximation. The numerical proportionality factor is of order unity and only increases modestly with smaller error tolerance.

## COMPUTATIONAL COST OF WINDOWING

We compare the accuracy of the simple cost function in the main text with the more elaborate and accurate

$$C_{elab} = \sum_l^{N_{vw}} \sum_m^{N_{cw}} N_{GL}^{lm}(N_c^{lm} + N_v^{lm})\,.$$

We choose a 2×2 windowing scheme so $N_{vw} = N_{cw} = 2$. We choose $N_{GL}^{lm}$ to give a maximum GL quadrature error of 0.5% for all transition energies in the $lm$ window (errors are quoted versus the simple estimator $\hat{P}_{lm}$ for that window pair). The global band gap is set to $E_{gap} = 0.5$ eV, the valence band is 12 eV wide, and the conduction band is 42 eV wide, making $E_{bw} = 54.5$ eV. (These energy parameters simulate bulk Si.) We set the number of valence and conduction bands to be 100 and 1000, respectively, and assume a flat density of states. The two free parameters in this example are the energy values $(E_v^*, E_c^*)$ that mark the boundary between the windows in the valence and conduction bands, respectively.

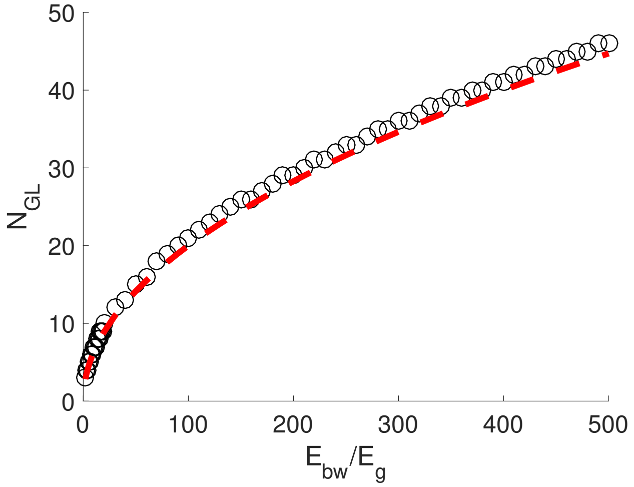


FIG. 2. Number of GL points ($N_{GL}$) needed as a function of $E_{bw}/E_g$ to achieve a fixed error of 0.1% in $\hat{P}$. 100 uniformly spaced valence band energies and 1000 uniformly spaced conduction band energies were sampled. The black circles show actual $N_{GL}$ values, while the red dashed line is the curve $2 \times \sqrt{E_{bw}/E_g}$.

Figure 3 shows the two cost functions as a function of the window sizes. The dimensionless axes are defined as $Ec_{ratio} = \frac{E_c^* - E_c^{min}}{E_c^{max} - E_c^*}$ and $Ev_{ratio} = \frac{E_v^* - E_v^{min}}{E_v^{max} - E_v^*}$, respectively. Ignoring the unimportant difference in vertical scale, we see that the simple estimator $C$ does a very good job of capturing the behavior of the more elaborate $C_{elab}$ cost function. Hence, we use the simpler cost function $C$ for our further considerations.

Using the simpler cost function $C$ (from the main text) for Si, we minimize the cost for each set of window numbers $N_{cw}$ and $N_{vw}$ going from 1 to 10 separately. This is done by considering the window boundaries to always ben chosen from a fixed list of energies that divide the valence or conduction bands into 10 equal segments. For a given number of windows $(N_{vw}, N_{cw})$, we minimize the cost function $C$ over all the discrete window choices. The band sampling has 100 and 1000 valence and conduction bands using a flat density of states. Figure 4 illustrates the resulting minimal cost as function of the number of windows which is smooth and favors a small number of windows. For this case, the minimum number of computation occurs at $N_{vw} = 1$ and $N_{cw} = 4$.

## DFT CALCULATION DETAILS

We perform DFT calculations to obtain the single particle wave functions and energies for the GW calculations. The plane wave pseudopotential supercell approach is used as implemented by the Quantum Espresso software package [1].

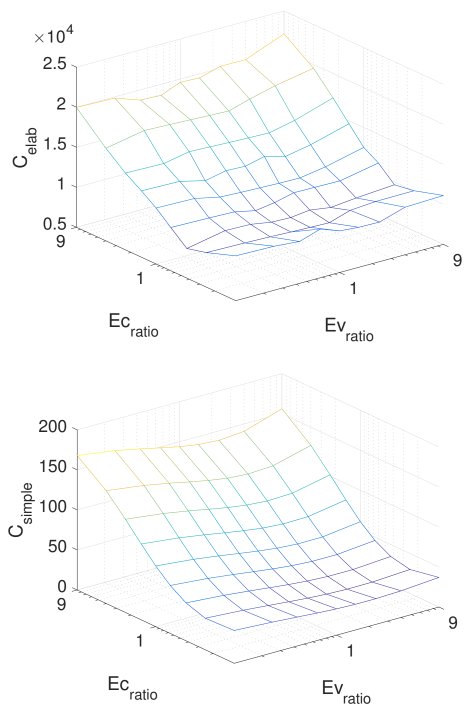


FIG. 3. Computational cost of windowing based on two cost functions. Top: computed cost based on the elaborate expression $C_{elab}$. Bottom: simple cost function $C$.

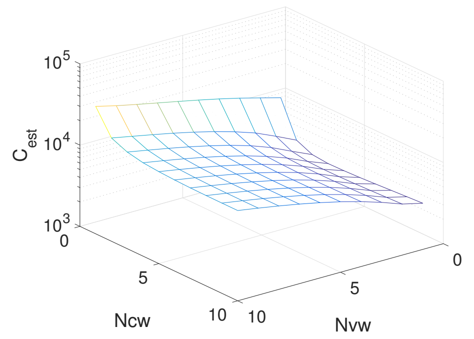


FIG. 4. Minimized computational cost function $C$ from the main text for Si for each set of number of windows $(N_{vw}, N_{cw})$.

For Si, we use the local density approximation (LDA) for exchange and correlation as parameterized by Perdew ad Zunger [2]. The Si norm-conserving pseudopotential is generated with the valence configuration of $3s^2 3p^2 3d^0$ with the cutoff radii of 1.75, 1.93, and 2.07 a.u. for $s$, $p$, and $d$ channels. The plane wave cutoff is 25 Ry, and the lattice parameter is fixed to the experimental one of 5.43 Å.

For MgO, GGA-PBE is used for the exchange-correlation functional [3]. Both Mg and O are represented by norm-conserving pseudopotentials generated with the valence configuration of $3s^2$ and $2s^2 2p^4 3d^0 4f^0$ for Mg and O, respectively. The plane wave cutoff is 50 Ry, and the lattice parameter is fixed to 8.42Å.

For the data in the main text on $\epsilon_\infty$ and the COHSEX band gap, we sample the gamma point of a 16 atom unit cell for both materials. For the $\mathrm{G_0W_0}$ band gaps for Si, a 4×4×4 sampling of the primitive cell equivalent to a 2×2×2 sampling of the 16 atom cell is used. The total number of bands was 399 for Si and 433 for MgO.

To create the data on computational load versus the number of atoms (Fig. 4 in the main text), we chose Si with the following number of $k$-point and bands: 52 bands with 8 k points for the 2-atom cell, 104 bands with 4 k points for the 4-atom cell, 208 bands with 2 k points for the 8-atom cell, and 416 bands with 1 k points for 16-atom cell.

## COMPUTING $P$ FOR METALS

As explained in the main text, the standard approach for dealing with metals is to use a smoothed step function $f(E)$ for the electron occupancies. Canonical examples include the Fermi-Dirac distribution

$$f(E) = \frac{1}{1 + \exp[\beta(E-\mu)]}$$

or the integral of a Gaussian

$$f(E) = \frac{\beta}{\sqrt{2\pi}} \int_E^\infty dx\, \exp(-[\beta(x-\mu)]^2/2)$$

where $\mu$ is the chemical potential and typical values of the broadening parameter $\beta$ which give highly converged results correspond to temperature well above ambient conditions (e.g., $\beta^{-1} = 0.1$ eV is typical). The static RPA irreducible polarizability matrix including the occupation function is

$$P_{r,r'} = -2 \sum_v^{N_v} \sum_c^{N_c} \frac{[f(E_v) - f(E_c)]\psi^*_{r,v}\psi_{r,c}\psi^*_{r',c}\psi_{r',v}}{E_c - E_v} \, .$$

The good news is that the energy-dependent part of the sum given by

$$\frac{f(E_v) - f(E_c)}{E_c - E_v}$$

is smooth for all energies and takes the finite value $-f'(\mu)$ when $E_v = E_c = \mu$. This means that all the terms in the sum for $P$ are finite and well behaved so the windowing and quadrature approach will work. Going through the derivation in the main text leads to minor changes in the final formula for $P$: as before we split $P$ into a sum over

window pairs

$$P_{r,r'} = \sum_{l}^{N_{vw}} \sum_{m}^{N_{cw}} P^{lm}_{r,r'}$$

while the contributions from each window pair are now given by

$$P^{lm}_{r,r'} = -\frac{2}{a_{lm}} \sum_{k=1}^{N^{lm}_{GL}} w_k \, e^{-x_k (E^{lm}_g / a_{lm} - 1)} \times \left\{ D^{lm}_{r,r'} E^{lm}_{r,r'} - F^{lm}_{r,r'} G^{lm}_{r,r'} \right\}$$

where

$$D^{lm}_{r,r'} = \sum_{v \in l} f(E_v) e^{-x_k \Delta E_{vl}/a_{lm}} \psi^*_{r,v} \psi_{r',v}$$

$$E^{lm}_{r,r'} = \sum_{c \in m} e^{-x_k \Delta E_{cm}/a_{lm}} \psi_{r,c} \psi^*_{r',c}$$

$$F^{lm}_{r,r'} = \sum_{v \in l} e^{-x_k \Delta E_{vl}/a_{lm}} \psi^*_{r,v} \psi_{r',v}$$

$$G^{lm}_{r,r'} = \sum_{c \in m} f(E_c) e^{-x_k \Delta E_{cm}/a_{lm}} \psi_{r,c} \psi^*_{r',c} \,.$$

All the matrices $D, E, F, G$ can be computed with $N_v N_r^2$ or $N_c N_r^2$ operations (i.e., cubic scaling) where $N_r$ is the number of $r$ grid points being used. Since $f(E_c)$ quickly becomes very small as a function of $E_c$, the second $FG$ term needs only be computed for the few window pairs where $\beta(E_c - \mu)$ is sufficiently small. Hence the added workload for dealing with a metal is quite modest.

## SPECIALIZED QUADRATURE FOR OVERLAPPING WINDOWS

As stated in the main text, the dynamic part of the GW self-energy matrix is given by

$$\begin{aligned} \Sigma(\omega)^{dyn}_{r,r'} &= \sum_{p,n} \frac{B^p_{r,r'} \psi_{rn} \psi^*_{r'n}}{\omega - \epsilon_n + sgn(\mu - \epsilon_n)\omega_p} \\ &= \sum_{p,v} \frac{B^p_{r,r'} \psi_{rv} \psi^*_{r'v}}{\omega - \epsilon_v + \omega_p} + \sum_{p,c} \frac{B^p_{r,r'} \psi_{rc} \psi^*_{r'c}}{\omega - \epsilon_c - \omega_p} \end{aligned} \quad (5)$$

where the matrices $B^p_{r,r'}$ are the residues and $\omega_p$ are the energies of the poles of the screened interaction $W(\omega)_{r,r'}$ while $c$ and $v$ label unoccupied (conduction) and occupied (valence) bands. We then form energy windows for the two energies $e_n = \omega - \epsilon_n$ and $\pm\omega_p$ entering the denominator. In direct correspondence to the windowing approach for the polarizability $P$ in the main text, we write

$$\Sigma(\omega)^{dyn}_{r,r'} = \sum_{l}^{N_{pw}} \sum_{m}^{N_{ew}} \Sigma^{lm}(\omega)_{r,r'}$$

where energy window $l$ contains the excitation energies $\Omega^{min}_l \le \pm\omega_p < \Omega^{max}_l$ and energy window $k$ contains the band energies satisfying $e^{min}_m \le e_n = \omega - \epsilon_n < e^{max}_m$. The notation $\pm\omega_p$ permits us to deal with both signs of $\omega_p$ in Eq. (5) in a unified manner. The contribution from window pair $(l, m)$ is

$$\Sigma^{lm}(\omega)_{r,r'} = \sum_{p \in l} \sum_{n \in m} \frac{B^p_{r,r'} \psi_{rn} \psi^*_{r'n}}{\omega - \epsilon_n \pm \omega_p}$$

Most pairs of windows $(l, m)$ have energy ranges that do not overlap, and thus the energy denominators in the sums for that window pair are never zero and have fixed sign for all terms. Hence, we can use the Gauss-Laguerre quadrature approach for the windows pair contribution $P^{lm}$ from the main text with no modifications.

The issue we discuss in this section involves dealing with the case where a pair of windows $(l, m)$ overlaps so that the denominator changes sign when the energy values are summed up over the window pairs. The Laplace transform and quadrature approach used for the polarizability is inapplicable for such cases. In the literature, this issue is dealt with by computing the principal part of the sums approximately. If $x = \omega - \epsilon_n \pm \omega_p$, one can either ignore contributions from small denominators [4] (i.e., setting $1/x$ to zero for small $x$) or use a smoothing function [5] that behaves as $1/x$ for large $x$ and smoothly goes to zero for small $x$ (e.g., replacing $1/x$ by $x/(\gamma^2 + x^2)$ with small $\gamma$).

Mathematically, what we seek is a good approximation to the function $1/(x + y)$, called $F(x + y)$, for the situation where $x + y$ can be both positive and negative. In addition, $F$ must have a separable form in $x$ and $y$ so that we can use it to separate the sums over $n$ and $p$ above to reduce the overall computational scaling. $F(x + y)$ should be an odd function of $x + y$ with finite values so that we can compute the principle part of the above sum about the divergence of the denominator without difficulties. Hence, for a pair of overlapping windows $(l, m)$, we will be computing

$$\Sigma^{lm}(\omega)_{r,r'} = \sum_{p \in l} \sum_{n \in m} B^p_{r,r'} \psi_{rn} \psi^*_{r'n} \, F(\omega - \epsilon_n \pm \omega_p) \,. \quad (6)$$

A standard choice in the literature for $F$ is to use a Lorentzian broadening parameter $\gamma > 0$:

$$F(x) = Im \frac{1}{\gamma - ix} = \frac{x}{x^2 + \gamma^2} \,. \quad (7)$$

This odd function is continuous, approximates $1/x$ when $|x| \gg \gamma$, and has a separable form as a Fourier integral

$$F(x) = Im\int_0^{\infty} e^{-\gamma u + iux}\, du = \frac{1}{\gamma}\, Im\int_0^{\infty} e^{-v} e^{ivx/\gamma}\, dv\,. \quad (8)$$

The exponential weight function here means the most appropriate quadrature method for approximating the integral is the usual Gauss-Laguerre quadrature for this case. Hence, this $F(x)$ can be used to separate the sums over $n$ and $p$ when computing $\Sigma^{dyn}$. The difficulties with this function are practical. First, the quadrature grids needed for reasonable errors can become large. Second, the function turns into $1/x$ only when $|x| \gg \gamma$ so that if $\gamma$ is not small compared to the width of the energy windows being employed, there will be sizable errors across window boundaries when we switch from using $F(x)$ to $1/x$. On the other hand, if we make $\gamma$ small to avoid this type of matching error, the steepness of $F(x)$ near the origin, directly related to the slow decay of $e^{-\gamma u}$ in the integral, requires a large quadrature grid.

We alleviate these difficulties by taking advantage of the freedom afforded in choosing the functional form of $F(x)$. We relate $F(x)$ to the weight function $w(v)$ via a Fourier integral based on an energy width $\delta$

$$F(x) = \frac{1}{\delta}\, Im \int_0^{\infty} w(v) e^{ivx/\delta}\, dv\,. \quad (9)$$

Choosing the weight $w(v) = e^{-v}$ recovers the above Lorentzian broadening function. After some trial and error, we find that a minimal change of the weight function is sufficient for our purposes. We propose the weight

$$w(v) = \exp(-v - v^2/2) \quad (10)$$

which falls off much faster for large $v$ and will thus generate a much smoother $F(x)$ for small $x$. However, since its behavior for small $v$ is the same as the $e^{-v}$, the associated $F(x)$ must also asymptote to $1/x$. Figure 5 shows a comparison of the weight functions and their computed Fourier transforms $F(x)$.

Generating an appropriate quadrature for this new weight function follows a standardized procedure in the theory of orthogonal polynomials [6]. The output of this procedure are a set of nodes $\{v_j\}$ and weights $\{w_j\}$ for each size of quadrature grid $n_q$ where $j = 1, 2, \ldots, n$. We then have the approximation

$$F(x) \approx \frac{1}{\delta} Im \sum_{j=1}^{n_q} w_j\, e^{iv_j x/\delta} = \frac{1}{\delta} \sum_{j=1}^{n_q} w_j\, \sin(v_j x/\delta)\,. \quad (11)$$

Table I shows how large the quadrature grid must be each specified maximum error for the Lorentzian generating weight $e^{-v}$ as well as the improved weight $\exp(-v - v^2/2)$ for an energy window of unit width. To generate this table, we specify a maximum percentage error and then find the broadening $\gamma$ or $\delta$ so that $F(x)$ differs from $1/x$ by less than the specified error when $x = 1$. We then find the size of a quadrature grid $n$ so that the difference between the quadrature approximation of Eq. (11) and the true $F(x)$ is below the desired error level for all $x$ in the window (i.e., $0 \le x \le 1$). It is clear that the new weight $\exp(-v - v^2/2)$ and associated quadrature is at least an order of magnitude more efficient than the standard weight $e^{-v}$.

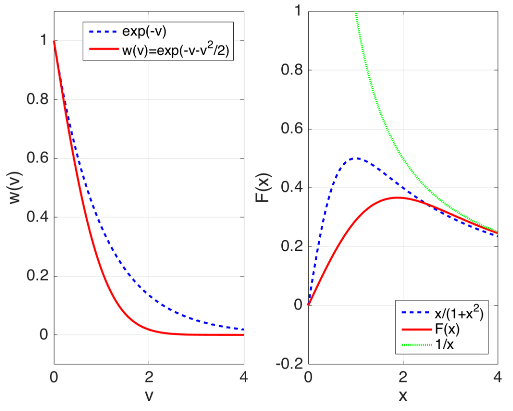


FIG. 5. Left: comparison of the two weight functions discussed in the text. The blue dashed curve is the exponential weight $\exp(-v)$ associated with the Lorentzian broadening approach; the solid red curve is the new proposed weighing function. Right: appropriate Fourier transforms of the weights. The exponential weight $e^{-v}$ (dashed blue) corresponds to $x/(1+x^2)$ while the weight $w(v) = \exp(-v - v^2/2)$ corresponds to $F(x)$ (solid red). For comparison, the target function $1/x$ is shown as well (short dashed green). $F(x)$ is smoother for small $x$ and appraoches $1/x$ more rapidly for large $x$ than $x/(1+x^2)$.

| % error | $n_q$ $(w = e^{-x})$ | $n_q$ $(w = e^{-x-x^2/2})$ |
|---|---|---|
| 5 | 6 | 1 |
| 1 | 24 | 1 |
| 0.1 | 124 | 5 |
| 0.01 | 547 | 15 |
| 0.001 | 2216 | 36 |

TABLE I. Size of quadrature grid needed for a maximum specified percent error for the two weight functions discussed in this section.

Finally, the use of the quadrature of Eq. (11) leads to the our desired separable form for the overlapping win-

dow pair $(l,m)$:

$$\Sigma^{lm}(\omega)^{dyn}_{r,r'} = \frac{1}{\delta}\sum_{j=1}^{n_q} w_j \Big\{ \left[\sum_{p\in l} B^p_{r,r'} \sin(\pm v_j\omega_p/\delta)\right] \times \left[\sum_{n\in m} \psi_{rn}\psi^*_{r'n} \cos(v_j(\omega-\epsilon_n)/\delta)\right] + \left[\sum_{p\in l} B^p_{r,r'} \cos(\pm v_j\omega_p/\delta)\right] \times \left[\sum_{n\in m} \psi_{rn}\psi^*_{r'n} \sin(v_j(\omega-\epsilon_n)/\delta)\right]\Big\}. \quad (12)$$

The nodes and weights can be found, for example, by using the two matlab functions provided below.

```
function [x,w]=GLquad(n)
% function [x,w]=GLagIntP(n)
% Gauss-Laguerre integration: return nodes x
% and weights w for a
% quadrature grid with n points

% This is basically the Golub-Welsch method
J=diag(1:2:2*n-1)+diag(1:n-1,1)+diag(1:n-1,-1);
[v,l]=eig(J);
[x,ix]=sort(diag(l));
w=v(1,ix)'.^2;
return

function [xmat,wmat] = myweightquad(n)
%function [xmat,wmat] = myweightquad(n)
% Return all nodes (xmat) and weights (wmat)
% for quadratures up to % n points for weight
% w(x)=exp(-x-x^2/2).  These are organized in
% matrices. xmat are the nodes and wmat
% are the weights.  Each column is for a
% quadrature size going from
% 1 to n (left to right).  Thus the lower
% triangle is padded with zeros.

% Figure out number of grid points
% so that the biggest moment (2n)
% is well converged.  We do
% Gauss-Laguerre quadrature to
% do these integrals over the weights!
Iold = 0;
for nx=round(10.^[1:.2:7])
    [xq,wq] = GLquad(nx);
    weight = exp(-xq.^2/2);
    I = sum(wq.*weight.*xq.^(2*n));
    if Iold>0
        err = (I-Iold)/I;
        if abs(err)<1e-14
            break
        end
    else
    end
    Iold = I;
end

% Build polynomials as we go
% and figure out the recursion
% relation coefficients as we go
p = zeros(length(xq),n+1);
p(:,1) = 1;
a = zeros(n,1);
b = zeros(n,1);
for j=1:n
    xpp = sum(wq.*xq.*weight.*p(:,j).^2);
    pp = sum(wq.*weight.*p(:,j).^2);
    a(j) = xpp/pp;
    if j>1
        ppm1 = sum(wq.*weight.*p(:,j-1).^2);
        b(j) = pp/ppm1;
    end
    if j>1
        p(:,j+1) = ...
            (xq-a(j)).*p(:,j)-b(j)*p(:,j-1);
    else
        p(:,j+1) = (xq-a(j)).*p(:,j);
    end
end

% Prepare for Golub-Welsch
b = b(2:end);
b = sqrt(b);
mu0 = sum(wq.*weight);

% Build Golub-Welsch J matrix,
% eigen decompose it, and get weights and
% nodes for each value of j=1,...,n
% (i.e. all weights and nodes for
% quadratures up to size n)
J = diag(a) + diag(b,1) + diag(b,-1);
xmat = zeros(n,n);
wmat = zeros(n,n);
for j=1:n
    Jcut = J(1:j,1:j);
    [v,d] = eig(Jcut);
    d = diag(d);
    [~,is] = sort(d);
    d = d(is);
    v = v(:,is);
    x = d;
    w = v(1,:).^2*mu0;
    w = w';
    xmat(:,j) = [x' zeros(1,n-j)]';
```

```
    wmat(:,j) = [w' zeros(1,n-j)]';
end

return
```

## PERFORMANCE TEST WITH PRIOR $O(N^4)$ AND $O(N^3)$ GW TECHNIQUES.

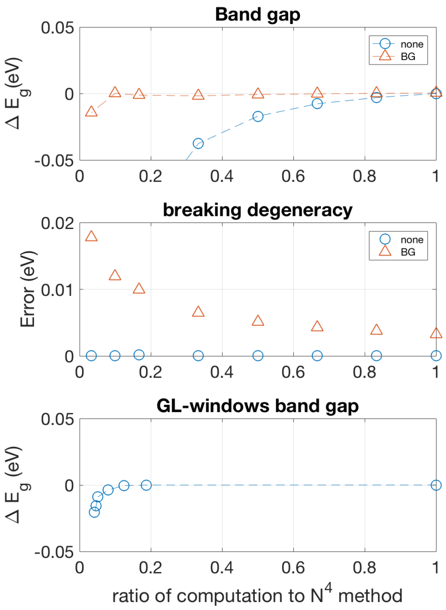


FIG. 6. Comparison between the $O(N^4)$ standard GW method, the $O(N^4)$ GW terminator method (BG [7]) implemented in Yambo code and the $O(N^3)$ windowed GL method for a 2-atom Si cell with 8 k points. (Top) Error in the $\Gamma - X$ band gap referenced to a calculation with 300 bands. The BG band gap is defined as the energy difference of the valence band maximum and the average of the conduction band minimum doublet. (Middle) The artificial degeneracy-breaking of the conduction band minimum doublet for Si. (Bottom) Error in band gap for our GL versus savings of computational work (see text for definition).

In this section, we compare GL quadrature method to existing quartic and cubic scaling GW methods to assess two important questions. First, does our windowed-GL $O(N^3)$ method offer computational advantages over available $O(N^4)$ methods for small systems? Second, is our method competitive with other existing $O(N^3)$ approaches?

We begin with a comparison to quartic methods, specifically with the accelerate $O(N^4)$ "terminator" approach [7] as implemented in the Yambo GW software (http://www.yambo-code.org/). A 2-atom Si cell with 8 k points is used to benchmark the behavior. Two terminator methods are implemented in Yambo, and we describe in detail the result based on the Bruneval and

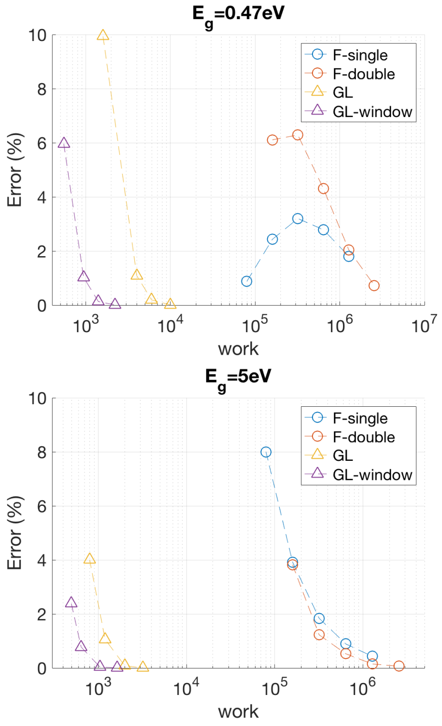


FIG. 7. Comparison between the cubic scaling Foerster et al. [9] and windowed GL methods. The y-axis is the error (%) of $\hat{P}$ for a 16-atom Si unit cell with 399 bands. The x-axis is the computational work needed to reach that accuracy: for the Foerster method it is $N_\omega(N_c + N_v)$ where $N_\omega$ is the number of frequency grid points and for the windowed GL method the workload is defined in the main text of the manuscript (Eq. 12). The band gap $E_{gap}$ is manually adjusted to investigate the effect of $E_{gap}$. F-single and F-double mean the Foerster method using single and double windows. GL and GL-window indicate Gauss-Laguerre quadrature method without and with multiple windows.

Gonze [7] method. (The Berger, Reining and Sottile [8] terminator method shows very similar results.) Fig. 6 shows the error in the band gap versus the computational savings using different number of bands for the self-energy $\Sigma$ calculation. The savings are referenced to a standard $O(N^4)$ no-terminator calculation with 300 bands which brings the converged band gap within 1 meV.

Both the $O(N^4)$ terminator method and the $O(N^3)$ GL method deliver more than 90% savings in the computational workload compared to the usual sum-over-states method when asking for an accuracy of 10 meV in the band gap of the 2-atom cell. The middle figure shows the artificial removal of the degeneracy of the conduction band minimum due to the user of terminators in Yambo (this may be a feature of the method or possibly an implementation issue in Yambo). We observe that the GL method is already competitive to the terminator method for this small system. Since our method scales cubically, it only becomes more efficient when the bigger size of sim-

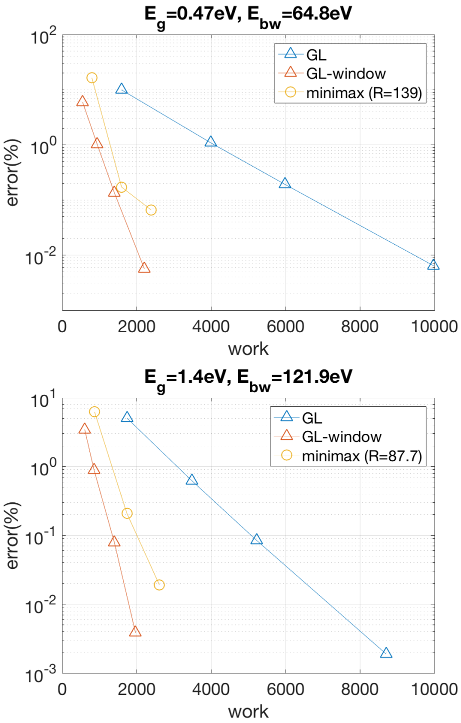


FIG. 8. Comparison between the cubic scaling minimax method of Liu et al. [10] and our windowed GL method for computation of $\hat{P}$. The computational work (x-axis) for the minimax method is $N_{grid}(N_c+N_v)$ where $N_{grid}$ is the number of imaginary time grid points.

ulation cell is used. We conclude that our cubic method has a sufficiently small prefactor to be competitive with accelerated GW methods even for small unit cells with less than 10 atoms.

Next, we compare our cubic scaling GL method to other existing cubic methods. Figures 7 and 8 compare the GL method to the performance of the cubic-scaling GW methods of Foerster et al. [9] and Liu et al. [10], respectively. We calculate $\hat{P}$ (eq. 4) with all three methods and examine the error versus computational workload.

In Fig. 7, we chose Si eigenvalues with 399 bands generated for 16-atom cell at the $\Gamma$ point. The work is defined as $N_\omega(N_c+N_v)$ where $N_\omega$ is a number of frequency grid points used in eq. 32 in Ref. [9]. To compare the windowing technique between Foerster et al. and ours, we calculate $\hat{P}$ with the single and double window methods of Foerster et al. To investigate the effect of the band gap on the windowing technique, we manually adjusted the band gap from 0.47 eV to 5 eV in the bottom figure (by uniformly shifting the conduction bands up in energy). Our main observation is that the Foerester et al. method is orders of magnitude more computationally expensive in comparison to our GL method (windowed or now) for the same level of accuracy.

Figure 8 shows the comparison between minimax grid technique (i.e., the approach of Liu et al.) and our GL quadrature method for computing $\hat{P}$. We used two sets of data, 399 Si eigenvalues from 16-atom cell and 435 MgO eigenvalues from 16-atom cell. For the minmax method, the computational work is defined as $N_{grid}(N_c+N_v)$ where $N_{grid}$ is the number of imaginary time grid points used in the minimax technique. We find that the minmax method is quite competitive, and always superior to GL quadrature without windows. However, once a windowed GL method is used, the comparison shifts in favor of our method.

* sohrab.ismail-beigi@yale.edu

[1] P. Giannozzi *et al.*, *J. Phys.: Cond. Matt.* **21**, 395502 (2009).
[2] J. P. Perdew and A. Zunger, *Phys. Rev. B* **23**, 5048 (1981).
[3] J. P. Perdew, K. Burke, M. Ernzerhof, *Phys. Rev. Lett.* **77**, 3865 (1996).
[4] Mark S. Hybertsen and Steven G. Louie, "Electron correlation in semiconductors and insulators: Band gaps and quasiparticle energies", *Physical Review B* **34** 5390 (1986).
[5] Deslippe, G. Samsonidze, D. A. Strubbe, M. Jain, M. L. Cohen and S. G. Louie, *Computer Physics Communications* **183**, 1269-1289, (2012). DOI 10.1016/j.cpc.2011.12.006
[6] Amparo Gil, Javier Segura, and Nico M. Temme, "5.3: Gauss quadrature" in *Numerical Methods for Special Functions*, SIAM, ISBN 978-0-89871-634-4 (2007).
[7] F. Bruneval and X. Gonze, *Phys. Rev. B* **78**, 085125 (2008).
[8] J. A. Berker, L. Reining, and F. Sottile, *Phys. Rev. B* **82**, 041103 (2010).
[9] D. Foerster, P. Koval, and D. Sanchez-Portal *J. Chem. Phys.* **135**, 074105 (2011).
[10] P. Liu, M. Kaltak, J. Klimes, and G. Kresse *Phys. Rev. B 94, 165109* **94**, 165109 (2016).
